# Supplementary material for: Rapid water diffusion at cryogenic temperatures through an inchworm-like mechanism
Source: arXiv:2112.13549 source file (2021-12-27)
Supplement: Supplementary file 1 [file SI_formatted.pdf]

# Supplementary Information: Rapid water diffusion at cryogenic temperatures through an inchworm-like mechanism

Wei Fang,[1,2] Kastur M. Meyer auf der Heide,[3] Christopher Zaum,[4] Angelos Michaelides,[5,1,*] and Karina Morgenstern[3,†]

[1]*Thomas Young Centre, London Centre for Nanotechnology, and Department of Physics and Astronomy, University College London, London WC1E 6BT, UK*

[2]*Laboratory of Physical Chemistry, ETH Zurich, CH-8093 Zurich, Switzerland*

[3]*Ruhr-Universität Bochum, Lehrstuhl für physikalische Chemie I, Universitätsstr. 150, D-44801 Bochum, Germany*

[4]*Leibniz Universität Hannover, Institut für Festkörperphysik, Appelstr. 2, D-30167 Hannover, Germany*

[5]*Yusuf Hamied Department of Chemistry, University of Cambridge, Lensfield Road, Cambridge CB2 1EW, UK*

In the supplementary information we provide additional experimental and simulation results. The contents are organised in the following order:

- I. Oligomers imaged with scanning tunnelling microscopy (STM) at enhanced contrast
- II. Rotatmers of the elongated water trimer imaged with STM
- III. Water trimer adsorption conformers predicted using density functional theory (DFT)
- IV. Transition between water trimer conformers
- V. Translational diffusion pathway of the water timer
- VI. Characterization of hydrogen bonds in the water trimer during the transition from elongated to cyclic trimer structures
- VII. Harmonic zero-point energy (ZPE) corrections, finite size corrections, and surface relaxation effects on the water trimer diffusion barriers
- VIII. Functional dependence of the water trimer diffusion barriers
- IX. Quantum tunneling contributions to the inchworm diffusion mechanism at low temperature
- X. Water monomer and dimer diffusion on metal (111) surface

## S.I. OLIGOMERS IMAGED AT ENHANCED CONTRAST

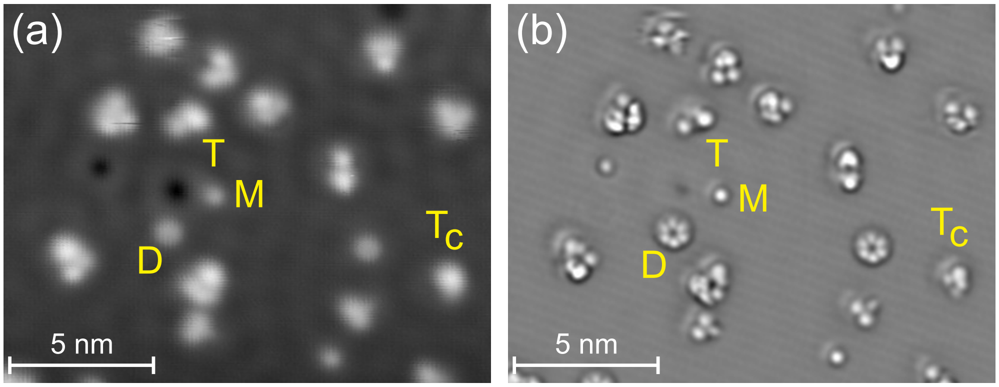


FIG. 1. Identification of trimers, 8.8 K, M: monomer, D: dimer, T: elongated trimer, $T_c$: circular trimer, STM images of same region of surface imaged by (a) conventional tip, 82 mV, 41 pA (b) modified tip, Laplace-filtered STM image, 82 mV, 35 pA.

The assignment of structures to trimers in the main manuscript is further corroborated by imaging them by a modified tip that is sharpened by an incidentally picked-up water molecule (Fig. 1). By this tip, the number of molecules in both, the elongated and circular protrusions is visualized, particularly well visible after a Laplace filtering (Fig. 1b). While monomers are still imaged as single protrusions (Fig. 1b, M), the images of the dimers (D) feature a sixfold symmetry by this tip, reflecting the six equivalent positions of the rotating upper molecule [1]. Note that this hexagonal structure is distinctly different from the hexagonally symmetric image of a hexamer by a metallic tip [2]. In particular, the distance between the protrusions differs. Here it is, at 0.45 nm, around only half the one of the hexamer in [2].

The objects of this study, the circular and the elongated trimers, consist indeed of three protrusions; one is brighter than the other two. The distances between the protrusions of the circular trimer ($T_c$ in Fig. 1b) are, at 0.42, 0.44, and 0.46 nm, rather similar, but larger than the interatomic distance of Cu(111) of 0.255 nm. For the elongated trimer ($T_e$ in Fig. 1b), the two outer molecules lead to well-separated protrusions, while the inner molecule is rather visible as an extended increase in apparent height. Also in this case, the distance between the two outer protrusions, is, at $(0.67 \pm 0.01)$ nm, considerably larger than the expected $\sqrt{3}$ distance of the Cu(111) surface of 0.44 nm. Such image distortion is, however, typical for

flexible molecular tips [3–6]. Regardless of these distortions, the number of imaged molecules corroborates our assignment of the elongated and circular protrusions with brighter corners to the elongated and circular trimers, respectively.

## S.II. POSSIBLE ROTAMERS AND ENANTIOMERS OF ASYMMTRIC ELONGATED TRIMER

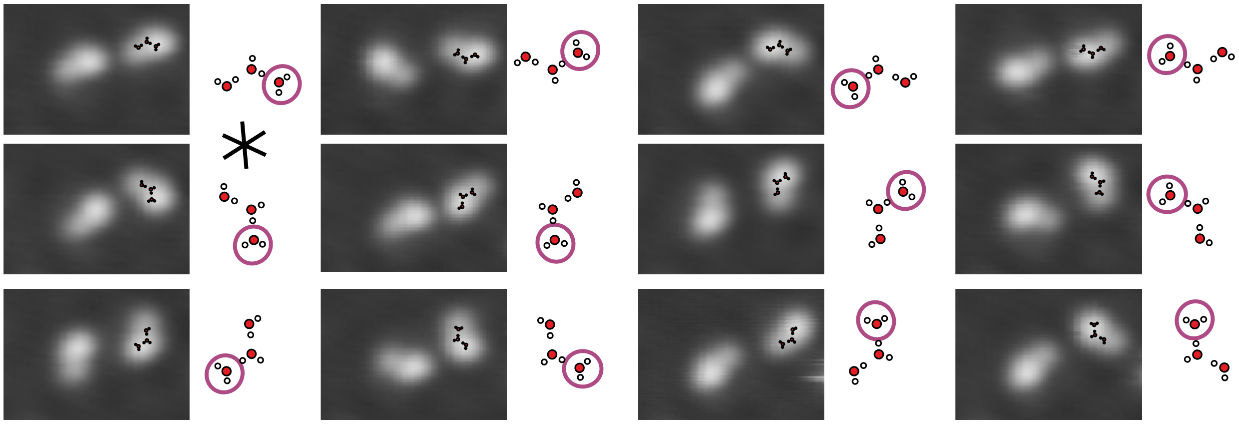

FIG. 2. Different forms of two elongated trimers with schematics superimposed to scale on the right trimer and displayed next to the STM images enlarged by a factor of two. The circles mark the molecules with larger height above the surface according to calculation. The six-way cross marks the ⟨110⟩ directions of Cu(111) as determined from images with atomic resolution.

The surface symmetry of an FCC(111) surface facilitates six rotamers of each of the two enantiomers for the elongated AD trimer; there should thus exist twelve different forms. Indeed, twelve different forms are observable for one trimer in course of 8 hours during which its motion was recorded at 7 K (Fig. 2). The possible rotamers of the two enantiomers fit thereby perfectly to the STM images.

## S.III. WATER TRIMER ADSORPTION GEOMETRIES ON CU(111) PREDICTED BY DFT

The six most stable water trimer conformers found in our DFT calculations are shown in Fig. 3. Among them, the most stable conformer is the elongated trimer ($T_e$), and the relative energy of the other conformers with respect to $T_e$ are given in Table I. $T_{e\text{-}2}$ has not

been observed in the experiment perhaps because it requires the water monomer to approach the donor water in the dimer, which is unlikely to happen as water dimers on the surface rapidly rotate about the donor water.

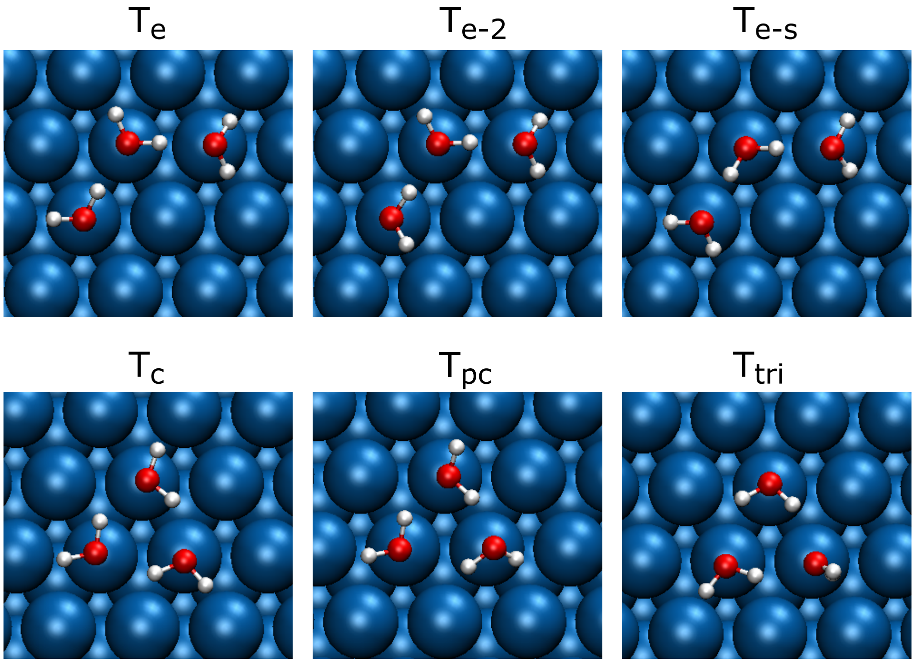


FIG. 3. Water trimer adsorption geometries found on Cu(111). $T_e$: elongated water trimer, $T_{e\text{-}2}$: form 2 of the elongated water trimer, $T_{e\text{-}s}$: elongated water trimer conformer with $C_s$ symmetry, $T_c$: cyclic water trimer, $T_{pc}$: pseudo-cyclic water trimer, $T_{tri}$: triangular water trimer.

| Geometry | Relative energy wrt $T_e$ (meV) | harmonic ZPE corrected (meV) |
|---|---|---|
| $T_{e\text{-}2}$ | 10 | 13 |
| $T_{e\text{-}s}$ | 20 | 9 |
| $T_c$ | 82 | 82 |
| $T_{pc}$ | 31 | 41 |
| $T_{tri}$ | 96 | - |

TABLE I. Relative energies of the water trimer conformers found with respect to the most stable conformer ($T_e$). The geometry of all the trimers are shown in Fig. 3. The harmonic zero point energy (ZPE) corrected values are also presented.

## S.IV. SWITCHING BETWEEN DIFFERENT CONFORMERS OF THE WATER TRIMER

The water trimer can switch between different conformers on the surface.

- Switching between $T_e$ and $T_{e\text{-}2}$ can happen through "wagging" of the donor (d) water. DFT calculations show that this process has a potential energy barrier of 61 meV.
- Switching between $T_e$ and $T_{e\text{-}s}$ can happen via a donor-acceptor exchange mechanism as shown in Fig. 4. The water trimer can effectively diffuse on the surface via this process, similar to the water dimer waltz diffusion mechanism [1, 7]. However, this process has a relatively high energy barrier of 300 meV for the water trimer on Cu(111), making it unfavorable compared to the other diffusion mechanisms. This is because the donor-acceptor exchange barrier is already relatively high for the water dimer on this surface (186 meV [7]), and that the H-bond strength (which correlates positively to this barrier [7]) is stronger in the trimer than in the dimer (as indicated by the O-O distance, which is 2.75 Å for the dimer and 2.7 Å for the trimer).
- Switching between $T_e$ and $T_c$ via $T_{pc}$ has been extensively discussed in the main text.
- Switching between $T_{e\text{-}2}$ and $T_{e\text{-}s}$ via $T_{tri}$. Note that the trimer cannot effectively diffuse on the surface via this mechanism, because the d water does not change in the process.

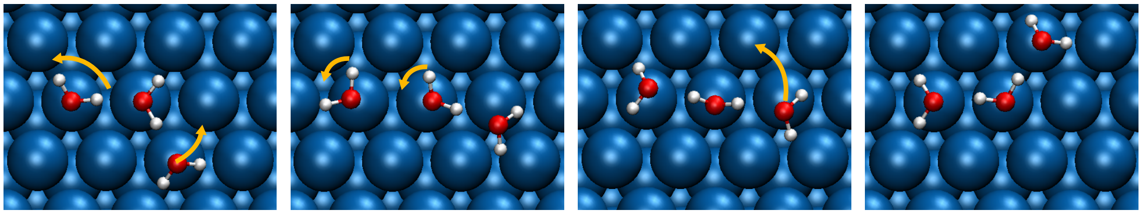

FIG. 4. Geometry of the donor-acceptor exchange process of the elongated water trimer on Cu(111). The second geometry is the transition state.

## S.V. TRANSLATIONAL DIFFUSION PATHWAY OF THE WATER TRIMER

The water trimer ($T_e$) translational diffusion pathway is shown in Fig. 5. In a step-wise manner, the d water molecule first moves to the bridge, then followed by the translation of

the entire water trimer water, similar to the water dimer translational diffusion mechanism [7, 8].

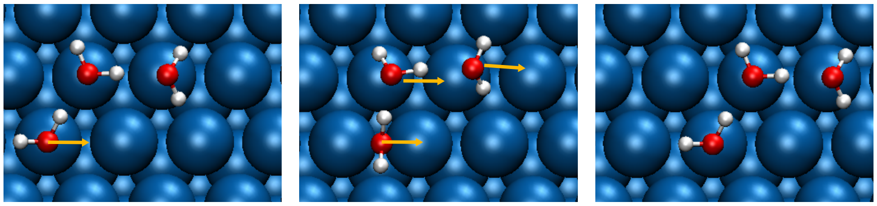

FIG. 5. Geometry of the donor-acceptor exchange process of the elongated water trimer on Cu(111).

## S.VI. CHARACTERIZATION OF H-BONDS IN THE WATER TRIMER DURING THE TRANSITION FROM ELONGATED TO CYCLIC TRIMER

To understand the stability of $T_{pc}$ and $T_c$, we show the O-O distance $d_{OO}$ and the H-bond bending angle change during the transition from $T_e$ to $T_c$ (Fig. 6). One can see that two H-bonds in $T_e$ bend and become less stable during the process, while a third H-bond forms and stabilizes the cluster.

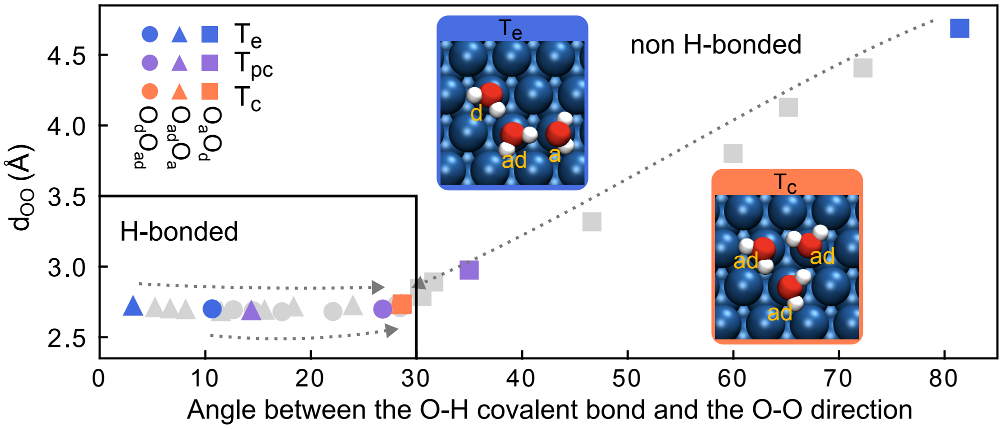


FIG. 6. Change of the O-O distance and bending angles during the transition from $T_e$ to $T_c$ via $T_{pc}$. The H-bond length is characterized by the O-O distance $d_{OO}$ and the bending angle is defined as $\alpha = \angle O_A\text{-}O_D\text{-}H_D$, where $O_D$ ($O_A$) is the O of the donor (acceptor) water, and $H_D$ is the H on the donor water that forms an acute angle with the $O_D$-$O_A$ direction. The light grey points are the other geometries along the NEB path. The solid black line marks the H-bond definition from Ref. 9.

We have also considered other geometrical H-bond characterization methods used for water. We find that 3 other definitions [10–12] also found that there are two H-bonds in $T_{pc}$ and three H-bonds in $T_c$, in agreement with the definition from Ref. 9. We note that there is a definition that has a stricter limit on the H-bond bending angle [13] predicts that only one H-bond in $T_{pc}$ qualifies as a H-bond and that $T_c$ has no H-bonds.

## S.VII. CORRECTIONS TO THE POTENTIAL ENERGY BARRIER

First we consider ZPE effects in the harmonic approximation. This correction is computed by taking the difference of the harmonic ZPE of the transition state and the reactant (Table II). We note that anharmonic ZPE effects could also be important, but due to the extremely low temperature in the experiment, such effects are very difficult to simulate.

Then we corrected for the finite size effects. We computed the energy barriers with the unit cell extended to a 10×8 supercell (with a 3×3×1 k-point mesh), with the geometries fixed at the optimized geometries obtained in a 5×4 unit cell. The corrections are obtained by taking the difference between the barriers in the large and small unit cell.

Next we considered the effects of flexible surface vs frozen surface. We reoptimized the adsorption geometries and transition state geometries with the first layer of the substrate flexible in the optimization. The surface relaxation correction is defined as the barrier difference computed with a frozen surface and a flexible surface.

Finally, we have also performed calculations with applied electric fields of ± 0.05 eV/Å. The geometries of the $T_e$ and $T_c$ have been re-optimized with the presence of the electric field. We found that the barrier for the inchworm diffusion mechanism changes from 82 meV to 89 meV (74 meV) for an electric field of +0.05 eV/Å (−0.05 eV/Å).

## S.VIII. EXAMINATION OF DFT FUNCTIONAL DEPENDENCE

Next we investigate the impact of the choice of DFT functional on the results. We tested 3 other functionals (including a meta-GGA functional) that accounts for the van der Waals interactions: optB86b-vdW [15], PBE-D3 [16, 17], and TPSS-D3 [17, 18]. The results are compared in Table III. Although the choice of DFT functional has a quantitative impact on the barriers (suggesting that it is difficult to obtain quantitatively accurate results for this

| | Inchworm | $T_e$ translation | $T_e$ rotation | $T_e$ to $T_{pc}$ |
|---|---|---|---|---|
| "Standard" Barrier (meV) | 82 | 118 | 35 | 31 |
| Harmonic ZPE correction (meV) | 0 | -19 | -9 | +10 |
| Finite size correction (meV) | -22 | +7 | +7 | -3 |
| Surface relaxation correction (meV) | +15 | +2 | +0 | +5 |
| "Corrected" Barrier (meV) | 75 | 108 | 33 | 43 |

TABLE II. DFT computed activation energy barriers for the key processes discussed in the text. Specifically, the following processes are considered: The inchworm diffusion process shown in Fig. 4 of the main text; A simple trimer translation process; Rotation of the $T_e$ trimer; Transition from the $T_e$ trimer to the $T_{pc}$ trimer. The harmonic ZPE correction, and finite size correction (the difference between the barrier computed in a large 10×8 unit cell and in a 5×4 unit cell), surface relaxation correction (the difference between the barrier computed with the first layer of substrate atoms fixed and optimized). Barriers are reported using the "standard" computational set-up (as described in the methods section of the main text) and "corrected" to take into account all the corrections above.

| DFT functional | Inchworm | $T_e$ to $T_{pc}$ | $T_e$ translation | $E(T_{e\text{-}2}) - E(T_e)$ |
|---|---|---|---|---|
| optB88-vdW [14] | 82 | 31 | 118 | 10 |
| optB86b-vdW [15] | 94 | 43 | 126 | 10 |
| PBE-D3 [16, 17] | 129 | 63 | 113 | 10 |
| TPSS-D3 [17, 18] | 124 | 73 | 134 | 8 |

TABLE III. DFT functional dependence of the potential energy barriers of the following processes: inchworm diffusion, transition to $T_{pc}$, and trimer translation. The functional dependence of the energy difference between $T_{e\text{-}2}$ and $T_e$ are also given. All units are in meV. The geometries are re-optimized for every functional.

system), the qualitative trend remains similar regardless of the choice of DFT functional.

## S.IX. QUANTUM TUNNELING IN THE INCHWORM DIFFUSION MECHANISM

Finally we consider quantum tunneling effects in the inchworm diffusion mechanism at low temperatures. As shown in the main text, the minimal energy pathway for this process features a so-called broad-top barrier. This is also supported by the fact that vibrational analysis of $T_c$ shows no imaginary mode. Upon estimating the crossover temperature from classical over-the-barrier hopping to quantum tunneling (using the definition designed for broad-top barriers [19]), we obtain a value of 16 K. Therefore we expect tunneling to play a role below 16 K. To obtain an idea of the tunneling pathway, we preformed ring-polymer instanton [20–22] optimizations at a temperature below the crossover temperature (10 K). Due to the complexity of the pathway and the exceedingly low temperature, instanton theory calculations become extremely challenging and we have so far only obtained preliminary insights (Fig. 7). Nevertheless, the results of the instanton calculations indicate that there is some heavy atom tunneling (of the oxygen atoms) and that this likely enhances water trimer diffusion at low temperatures.

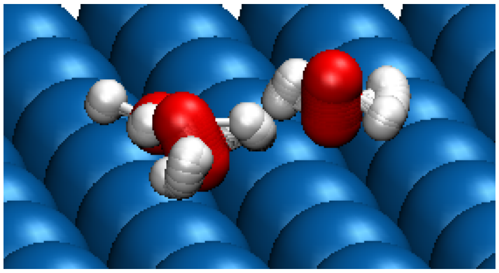

FIG. 7. Geometry of the instanton at 10 K with 34 ring-polymer beads, with total force optimized to below 0.8 eV/Å.

To estimate the tunneling contributions to the trimer diffusion rate, we resort to using the minimal energy pathway as a 1 dimensional model for this process and the WKB approximation [23], which is more crude and approximate but feasible for this system. We predict that tunneling increases the rate by 20 fold at 15 K, and by 8 orders of magnitude at 10 K. This means that tunneling (of the heavy oxygen atoms) does indeed contribute to increasing the diffusivity of the water trimer at low temperatures. However, tunneling alone is not enough to bridge the gap between experimental observation and theory as the rate for the inchworm diffusion is still too low to be observed at these temperatures ($<$ 1E-10 $s^{-1}$) even after accounting for tunneling effects. A full study of the importance of quantum

nuclear effects is beyond the scope of the current article.

## S.X. WATER MONOMER AND DIMER DIFFUSION ON METAL (111) SURFACE

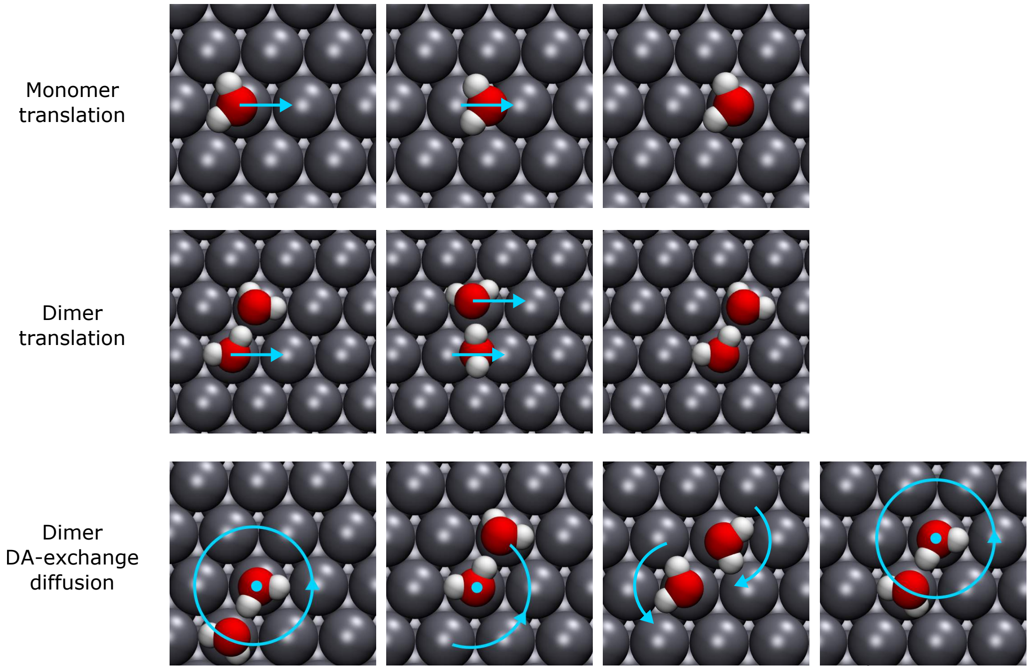


FIG. 8. Top view of the water monomer translation, dimer translation, and dimer donor-acceptor (DA) exchange diffusion pathways on transition metal (111) surfaces.

* am452@cam.ac.uk
† karina.morgenstern@rub.de

[1] V. A. Ranea, A. Michaelides, R. Ramirez, P. L. de Andres, J. A. Verges, and D. A. King, "Water dimer diffusion on Pd(111) assisted by an h-bond donor-acceptor tunneling exchange," Phys. Rev. Lett. **92**, 136104 (2004).

[2] A. Michaelides and K. Morgenstern, "Ice nanoclusters at hydrophobic metal surfaces," Nat. Mater. **6**, 597–601 (2007).

[3] P. Hapala, G. Kichin, C. Wagner, F.S. Tautz, R. Temirov, and P. Jelinek, " mechanism of high-resolution stm/afm imaging with functionalized tips," Phys. Rev. B **90**, 085421 (2014).

[4] N. Moll, B. Schuler, S. Kawai, F. Xu, L. Peng, A. Orita, J. Otera, A. Curioni, M. Neu, J. Repp, G. Meyer, and L. Gross, "Image distortions of a partially fluorinated hydrocarbon molecule in atomic force microscopy with carbon monoxide terminated tips," Nano Lett. **14**, 6127–6131 (2014).

[5] M. Emmrich, F. Huber, F. Pielmeier, J. Welker, T. Hofmann, M. Schneiderbauer, D. Meuer, S. Polesya, S. Mankovsky, D. Ködderitzsch, H. Ebert, and F.J. Giessibl, "Subatomic resolution force microscopy reveals internal structure and adsorption sites of small iron clusters," Science **348**, 308–311 (2015).

[6] C.-S. Guo, X. Xin, M.A. Van Hove, X. Ren, and Y. Zhao, "Origin of the contrast interpreted as intermolecular and intramolecular bonds in atomic force microscopy images," J. Phys. Chem. **119**, 14195–14200 (2015).

[7] Wei Fang, Ji Chen, Philipp Pedevilla, Xin-Zheng Li, Jeremy O Richardson, and Angelos Michaelides, "Origins of fast diffusion of water dimers on surfaces," Nat. Comm. **11**, 1689 (2020).

[8] C. Bertram, K. Morgenstern, P. Pedevilla, and A. Michaelides, "Anomalously low barrier for water dimer diffusion on Cu(111)," Nano Lett. **19**, 3049–3056 (2019).

[9] A. Luzar and D. Chandler, "Hydrogen-bond kinetics in liquid water," Nature **379**, 55–57 (1996).

[10] Ph. Wernet, D. Nordlund, U. Bergmann, M. Cavalleri, M. Odelius, H. Ogasawara, L. Å. Näslund, T. K. Hirsch, L. Ojamäe, P. Glatzel, L. G. M. Pettersson, and A. Nilsson, "The

structure of the first coordination shell in liquid water," Science **304**, 995–999 (2004).

[11] Teodora Todorova, Ari P. Seitsonen, JÃ¼rg Hutter, I-Feng W. Kuo, and Christopher J. Mundy, "Molecular dynamics simulation of liquid water: Hybrid density functionals," J. Phys. Chem. B **110**, 3685–3691 (2006).

[12] Alenka Luzar, "Resolving the hydrogen bond dynamics conundrum," J. Chem. Phys. **113**, 10663–10675 (2000).

[13] I-Feng W. Kuo and Christopher J. Mundy, "An ab initio molecular dynamics study of the aqueous liquid-vapor interface," Science **303**, 658–660 (2004).

[14] J. Klimeš, David R Bowler, and Angelos Michaelides, "Chemical accuracy for the van der Waals density functional," J. Phys. Condens. Matter **22**, 022201–1–5 (2010).

[15] J. Klimeš, David R. Bowler, and Angelos Michaelides, "Van der Waals density functionals applied to solids," Phys. Rev. B **83**, 195131 (2011).

[16] John P. Perdew, Kieron Burke, and Matthias Ernzerhof, "Generalized gradient approximation made simple," Phys. Rev. Lett. **77**, 3865–3868 (1996).

[17] Stefan Grimme, Stephan Ehrlich, and Lars Goerigk, "Effect of the damping function in dispersion corrected density functional theory," J. Comput. Chem. **32**, 1456–1465 (2011).

[18] Jianmin Tao, John P. Perdew, Viktor N. Staroverov, and Gustavo E. Scuseria, "Climbing the density functional ladder: Nonempirical meta˘generalized gradient approximation designed for molecules and solids," Phys. Rev. Lett. **91**, 146401 (2003).

[19] Wei Fang, Jeremy O. Richardson, Ji Chen, Xin-Zheng Li, and Angelos Michaelides, "Simultaneous deep tunneling and classical hopping for hydrogen diffusion on metals," Phys. Rev. Lett. **119**, 126001 (2017).

[20] Stefan Andersson, Gunnar Nyman, Andri Arnaldsson, Uwe Manthe, and Hannes Jónsson, "Comparison of quantum dynamics and quantum transition state theory estimates of the H + $CH_4$ reaction rate," J. Phys. Chem. A **113**, 4468–4478 (2009).

[21] Jeremy O. Richardson, "Ring-polymer instanton theory," Int. Rev. Phys. Chem. **37**, 171–216 (2018).

[22] Johannes Kästner, "Theory and simulation of atom tunneling in chemical reactions," WIREs: Comput. Mol. Sci. **4**, 158–168 (2014).

[23] R. P. Bell, *Tunnel Effect in Chemistry* (Chapman & Hall, 1980).
